# Supplementary material for: Tackling Catastrophic Forgetting and Background Shift in Continual Semantic Segmentation
Source: arXiv:2106.15287 source file (2021-06-29)
Supplement: Supplementary file 1 [file supplementary.tex]

\appendix
\section{Appendix}

\subsection{Further Work}

In our CSS setting, pixels of task $T$ can belong to old $C^{1:t-1}$, current $C^t$, and future classes $C^{t+1:T}$. In this paper we cover how to better handle old and current classes. Further works should investigate how to exploit the already present future information with Zeroshot \cite{lampert2009zeroshot,kumar2018synthesized_zeroshot} as already done in semantic segmentation \cite{kato2019zeroshotsegmentation,bucher2019zeroshotsegmentation} and explored for continual classification \cite{wang2020bookworm,douillard2020ghost}.

\subsection{Algorithm view of Local POD}

In \autoref{algo:local_pod}, we summarize the algorithm for the proposed Local POD. The algorithm consists in three functions. First, \texttt{Distillation}, loops over all $L$ layers onto which we apply Local POD. Second, \texttt{LocalPOD}, computes the L2 distance (L.26) between POD embeddings of the current (L.19) and old (L.20) models. It loops over $S$ different scales (L.14) and $\Phi$ computes the POD embedding given two features maps subsets (L.19-20) as defined in Eq. 1. $\|=$ denotes an in-place concatenation.

\input{algo/localpod}

\subsection{Reproducibility}

\noindent\textbf{Datasets:\,} We evaluate our model on three datasets Pascal-VOC~\cite{everingham2015pascalvoc}, ADE20k~\cite{zhou2017adedataset}, and Cityscapes~\cite{cordts2016cityscapes}. VOC contains 20 classes, 10,582 training images, and 1,449 testing images. ADE20k has 150 classes, 20,210 training images, and 2,000 testing images. Cityscapes contains 2975 and 500 images for train and test, respectively. Those images represent 19 classes and were taken from 21 different cities. All ablations and hyperparameters tuning were done on a validation subset of the training set made of 20\% of the images. 
For all datasets, we resize the images to $512 \times 512$, with a center crop. An additional random horizontal flip augmentation is applied at training time.

\noindent\textbf{Implementation details:\,} For all experiments, we use a Deeplab-V3~\cite{chen2017deeplabv3} architecture with a ResNet-101~\cite{he2016resnet} backbone pretrained on ImageNet~\cite{deng2009imagenet}, as in~\cite{cermelli2020modelingthebackground}. For all datasets, we set a maximum threshold for the uncertainty measure of Eq. 7 to $\tau=1e-3$. We train our model for 30 and 60 epochs per CSS step on Pascal VOC and ADE, respectively, with an initial learning rate of $1e-2$ for the first CSS step, and $1e-3$ for all the following ones. We reduce the learning rate exponentially with a decay rate of $9e-1$. We use SGD optimizer with $9e-1$ Nesterov momentum. The Local POD factor $\lambda$ is set to $1e-2$ and $5e-4$ for intermediate feature maps and logits, respectively. Moreover, we multiply this factor by the adaptive weighting $\sqrt{\nicefrac{|C^{1:t}|}{|C^{t}|}}$ introduced by \cite{hou2019ucir} that increases the strength of the distillation the further we are into the continual process. For all feature maps, Local POD is applied before ReLU, with squared pixel values, as in \cite{zagoruyko2016distillation_attention,douillard2020podnet}. We use 3 scales for Local POD: $1$, $\nicefrac{1}{2}$, and $\nicefrac{1}{4}$, as adding more scales experimentally brought diminishing returns. We use a batch size of 24 distributed on two GPUs. Contrary to many continual models, we don't have access to any task id in inference, therefore our setting/strategy has to predict a class among the set of all seen classes ---a realist setting.

% \subsection{Classes ordering details}

\noindent\textbf{Classes ordering details:\,} For all quantitative experiments on Pascal-VOC 2012 and ADE20k, the same class ordering was used across all evaluated models. For Pascal-VOC 2012 it corresponds to \lstinline![1, 2, ..., 20]! and ADE20k to \lstinline![1, 2, ..., 150]! as defined in \cite{cermelli2020modelingthebackground}. For continual-domain cityscapes, the order of the domains/cities is the following: \texttt{aachen}, \texttt{bremen}, \texttt{darmstadt}, \texttt{erfurt}, \texttt{hanover}, \texttt{krefeld}, \texttt{strasbourg}, \texttt{tubingen}, \texttt{weimar}, \texttt{bochum}, \texttt{cologne}, \texttt{dusseldorf}, \texttt{hamburg}, \texttt{jena}, \texttt{monchengladbach}, \texttt{stuttgart}, \texttt{ulm}, \texttt{zurich}, \texttt{frankfurt}, \texttt{lindau}, and \texttt{munster}.

In the main paper we showcased a boxplot featuring 20 different class orders for Pascal-VOC 2012 15-1. For the sake of reproducibility, we provide details on these orders:

\begin{adjustbox}{width=\columnwidth,center}
\begin{lstlisting}
[1, 2, 3, 4, 5, 6, 7, 8, 9, 10, 11, 12, 13, 14, 15, 16, 17, 18, 19, 20]
[12, 9, 20, 7, 15, 8, 14, 16, 5, 19, 4, 1, 13, 2, 11, 17, 3, 6, 18, 5]
[9, 12, 13, 18, 2, 11, 15, 17, 10, 8, 4, 5, 20, 16, 6, 14, 19, 1, 7, 3]
[13, 19, 15, 17, 9, 8, 5, 20, 4, 3, 10, 11, 18, 16, 7, 12, 14, 6, 1, 2]
[15, 3, 2, 12, 14, 18, 20, 16, 11, 1, 19, 8, 10, 7, 17, 6, 5, 13, 9, 4]
[7, 13, 5, 11, 9, 2, 15, 12, 14, 3, 20, 1, 16, 4, 18, 8, 6, 10, 19, 17]
[12, 9, 19, 6, 4, 10, 5, 18, 14, 15, 16, 3, 8, 7, 11, 13, 2, 20, 17, 1]
[13, 10, 15, 8, 7, 19, 4, 3, 16, 12, 14, 11, 5, 20, 6, 2, 18, 9, 17, 1]
[3, 14, 13, 1, 2, 11, 15, 17, 7, 8, 4, 5, 9, 16, 19, 12, 6, 18, 10, 20]
[1, 14, 9, 5, 2, 15, 8, 20, 6, 16, 18, 7, 11, 10, 19, 3, 4, 17, 12, 13]
[16, 13, 1, 11, 12, 18, 6, 14, 5, 3, 7, 9, 20, 19, 15, 4, 2, 10, 8, 17]
[10, 7, 6, 19, 16, 8, 17, 1, 14, 4, 9, 3, 15, 11, 12, 2, 18, 20, 13, 5]
[7, 5, 3, 9, 13, 12, 14, 19, 10, 2, 1, 4, 16, 8, 17, 15, 18, 6, 11, 20]
[18, 4, 14, 17, 12, 10, 7, 3, 9, 1, 8, 15, 6, 13, 2, 5, 11, 20, 16, 19]
[5, 4, 13, 18, 14, 10, 19, 15, 7, 9, 3, 2, 8, 16, 20, 1, 12, 11, 6, 17]
[9, 12, 13, 18, 7, 1, 15, 17, 10, 8, 4, 5, 20, 16, 6, 14, 19, 11, 2, 3]
[3, 14, 13, 18, 2, 11, 15, 17, 10, 8, 4, 5, 20, 16, 6, 12, 19, 1, 7, 9]
[7, 5, 9, 1, 15, 18, 14, 3, 20, 10, 4, 19, 11, 17, 16, 12, 8, 6, 2, 13]
[3, 14, 6, 1, 2, 11, 12, 17, 7, 20, 4, 5, 9, 16, 19, 15, 13, 18, 10, 8]
[1, 2, 12, 14, 6, 19, 18, 17, 5, 20, 8, 4, 9, 16, 10, 3, 15, 13, 11, 7]
\end{lstlisting}
\end{adjustbox}

In the 15-1 setting, we first learn the first fifteen classes, then increment the five remaining classes one by one. Note that the special class \texttt{background} (0) is always learned during the first task.

\noindent\textbf{Hardware and Code:\,} For each experiment, we used two Titan Xp GPUs with 12 Go of VRAM each. The initial step $t=1$ for each setting is common to all models, therefore we re-use the weights trained on this step. All models took less than 2 hours to train on Pascal-VOC 2012 15-1, and less than 16 hours on ADE20k 100-10. We distributed the batch size equally on both GPUs. All models are implemented in PyTorch~\cite{paszke2017pytorch} and runned with half-precision for efficiency reasons with Nvdia's APEX library (\href{https://github.com/NVIDIA/apex}{https://github.com/NVIDIA/apex}) using O1 optimization level. Our code base is based on \cite{cermelli2020modelingthebackground}'s code (\href{https://github.com/fcdl94/MiB}{https://github.com/fcdl94/MiB}) that we modified to implement our strategy. It is available at \href{https://github.com/arthurdouillard/CVPR2021_PLOP}{https://github.com/arthurdouillard/CVPR2021\_PLOP}.

\subsection{Additional Experiments}

\noindent\textbf{Model ablation:\,} \autoref{tab:ablation} shows the construction of our model component by component on Pascal-VOC 2012 in 15-5 and 15-1. For this experiment, we train our model on 80\% of the training set and evaluate on the validation set made of the remaining 20\%. We report the mIoU at the final task (``\textit{all}'') and the average of the mIoU after each task (``\textit{avg}'').
We start with a crude baseline made of solely cross-entropy (CE). Pseudo-labeling by itself increases by a large margin performance (eg. 3.99 to 19.74 for 15-1). Applying Local POD reduces drastically the forgetting leading to a massive gain of performance (eg. 19.74 to 50.41 for 15-1). Finally our adaptive factor $\nu$ based on the ratio of accepted pseudo-labels over the number of background pixels further increases our overall results (eg. 50.41 to 52.31 for 15-1). The interest of $\nu$ arises when PLOP faces hard images where few pseudo-labels will be created due to an overall high uncertainty. In such a case, current classes will be over-represented, which can in turn lead to strong bias towards new classes (\textit{i.e.} the model will have a tendency to predict one of the new classes for every pixel). The $\nu$ factor therefore decreases the overall classification loss on such images, and empirical results confirm its effectiveness.

\input{tables/ablations}

%\noindent\textbf{Scales Ablations:\,} \autoref{tab:ablation_scales} showcases an ablation of the different scales of Local POD. For this study, we apply the loss only on the backbone to have a fair comparison with the base POD. The smallest scale ($\nicefrac{1}{4}$) results in the best individual performance, and adding all three scales together produces our final Local POD. For simplicity, we also set the same scales ($1 \& \nicefrac{1}{2} \& \nicefrac{1}{4}$) for the logits. For the logits, we sum the channels associated with the new classes with the background channel in order to match the logits of the previous model.

%\input{tables/ablation_scales}

\noindent\textbf{Pascal-VOC 2012 Disjoint:\,} In the main paper, we reported results on Pascal-VOC 2012 Overlap. For reasons mentioned previously, Overlap is a more realist setting than Disjoint. Nevertheless, for the sake of comparison, we also provide results in \autoref{tab:voc_disjoint_sota} in the Disjoint setting.
While PLOP has similar performance to MiB in 15-5 (the differences are not significant), it significantly outperforms previous state-of-the-art methods in both 19-1 and 15-1.

\input{tables/voc_disjoint}
%\input{tables/ade_disjoint}

\noindent\textbf{Pascal-VOC 2012 Overlap with more baselines:\,} In \autoref{tab:voc_sota_full}, we report results on Pascal-VOC 2012 Overlap with more baselines. In addition to the models presented in the main paper, we add a naive Fine Tuning, two continual models based on weights constraints (PI \cite{zenke2017synaptic_intelligence} and RW \cite{chaudhry2018riemannien_walk}), and one continual model based on knowledge distillation (LwF \cite{li2018lwf}). PLOP surpasses these methods in all CSS scenarios. 

\input{tables/voc_full}

%\input{tables/pseudo_ablations}
